# Supplementary material for: Integrated Balanced and Staggered Routing in Autonomous Mobility-on-Demand Systems
Source: arXiv:2506.19722 source file (2025-06-24)
Supplement: Supplementary file 1 [file absolute_max_deviation_minutes_histogram.tex]

% This file was created with tikzplotlib v0.10.1.
\begin{tikzpicture}

\definecolor{darkgray176}{RGB}{176,176,176}
\definecolor{darkorange}{RGB}{255,140,0}

\begin{axis}[
height=\InstancesHistogramsHeight,
minor xtick={},
minor ytick={},
scaled y ticks=true,
tick align=outside,
tick pos=left,
width=\InstancesHistogramsWidth,
x grid style={darkgray176},
xlabel={[min]},
xmin=-0.9, xmax=8.6205,
xtick style={color=black},
xtick={-2,0,2,4,6,8,10},
xticklabel style={/pgf/number format/fixed, /pgf/number format/precision=0},
y grid style={darkgray176},
y tick label style={/pgf/number format/sci, /pgf/number format/sci zerofill=false},
ymin=0, ymax=24245.55,
ytick style={color=black},
ytick={0,5000,10000,15000,20000,25000},
yticklabel style={/pgf/number format/sci, /pgf/number format/precision=0},
yticklabels={0.0,0.5,1.0,1.5,2.0,2.5}
]
\draw[draw=black,fill=darkorange,opacity=0.7,line width=0.48pt] (axis cs:0,0) rectangle (axis cs:0.1642,1472);
\draw[draw=black,fill=darkorange,opacity=0.7,line width=0.48pt] (axis cs:0.1642,0) rectangle (axis cs:0.3284,3129);
\draw[draw=black,fill=darkorange,opacity=0.7,line width=0.48pt] (axis cs:0.3284,0) rectangle (axis cs:0.4926,6371);
\draw[draw=black,fill=darkorange,opacity=0.7,line width=0.48pt] (axis cs:0.4926,0) rectangle (axis cs:0.6568,10309);
\draw[draw=black,fill=darkorange,opacity=0.7,line width=0.48pt] (axis cs:0.6568,0) rectangle (axis cs:0.821,14105);
\draw[draw=black,fill=darkorange,opacity=0.7,line width=0.48pt] (axis cs:0.821,0) rectangle (axis cs:0.9852,23091);
\draw[draw=black,fill=darkorange,opacity=0.7,line width=0.48pt] (axis cs:0.9852,0) rectangle (axis cs:1.1494,16663);
\draw[draw=black,fill=darkorange,opacity=0.7,line width=0.48pt] (axis cs:1.1494,0) rectangle (axis cs:1.3136,18661);
\draw[draw=black,fill=darkorange,opacity=0.7,line width=0.48pt] (axis cs:1.3136,0) rectangle (axis cs:1.4778,20031);
\draw[draw=black,fill=darkorange,opacity=0.7,line width=0.48pt] (axis cs:1.4778,0) rectangle (axis cs:1.642,14649);
\draw[draw=black,fill=darkorange,opacity=0.7,line width=0.48pt] (axis cs:1.642,0) rectangle (axis cs:1.8062,11057);
\draw[draw=black,fill=darkorange,opacity=0.7,line width=0.48pt] (axis cs:1.8062,0) rectangle (axis cs:1.9704,10970);
\draw[draw=black,fill=darkorange,opacity=0.7,line width=0.48pt] (axis cs:1.9704,0) rectangle (axis cs:2.1346,7497);
\draw[draw=black,fill=darkorange,opacity=0.7,line width=0.48pt] (axis cs:2.1346,0) rectangle (axis cs:2.2988,4835);
\draw[draw=black,fill=darkorange,opacity=0.7,line width=0.48pt] (axis cs:2.2988,0) rectangle (axis cs:2.463,6179);
\draw[draw=black,fill=darkorange,opacity=0.7,line width=0.48pt] (axis cs:2.463,0) rectangle (axis cs:2.6272,4146);
\draw[draw=black,fill=darkorange,opacity=0.7,line width=0.48pt] (axis cs:2.6272,0) rectangle (axis cs:2.7914,2926);
\draw[draw=black,fill=darkorange,opacity=0.7,line width=0.48pt] (axis cs:2.7914,0) rectangle (axis cs:2.9556,2448);
\draw[draw=black,fill=darkorange,opacity=0.7,line width=0.48pt] (axis cs:2.9556,0) rectangle (axis cs:3.1198,1375);
\draw[draw=black,fill=darkorange,opacity=0.7,line width=0.48pt] (axis cs:3.1198,0) rectangle (axis cs:3.284,1404);
\draw[draw=black,fill=darkorange,opacity=0.7,line width=0.48pt] (axis cs:3.284,0) rectangle (axis cs:3.4482,1642);
\draw[draw=black,fill=darkorange,opacity=0.7,line width=0.48pt] (axis cs:3.4482,0) rectangle (axis cs:3.6124,678);
\draw[draw=black,fill=darkorange,opacity=0.7,line width=0.48pt] (axis cs:3.6124,0) rectangle (axis cs:3.7766,168);
\draw[draw=black,fill=darkorange,opacity=0.7,line width=0.48pt] (axis cs:3.7766,0) rectangle (axis cs:3.9408,504);
\draw[draw=black,fill=darkorange,opacity=0.7,line width=0.48pt] (axis cs:3.9408,0) rectangle (axis cs:4.105,178);
\draw[draw=black,fill=darkorange,opacity=0.7,line width=0.48pt] (axis cs:4.105,0) rectangle (axis cs:4.2692,47);
\draw[draw=black,fill=darkorange,opacity=0.7,line width=0.48pt] (axis cs:4.2692,0) rectangle (axis cs:4.4334,125);
\draw[draw=black,fill=darkorange,opacity=0.7,line width=0.48pt] (axis cs:4.4334,0) rectangle (axis cs:4.5976,48);
\draw[draw=black,fill=darkorange,opacity=0.7,line width=0.48pt] (axis cs:4.5976,0) rectangle (axis cs:4.7618,3);
\draw[draw=black,fill=darkorange,opacity=0.7,line width=0.48pt] (axis cs:4.7618,0) rectangle (axis cs:4.926,8);
\draw[draw=black,fill=darkorange,opacity=0.7,line width=0.48pt] (axis cs:4.926,0) rectangle (axis cs:5.0902,14);
\draw[draw=black,fill=darkorange,opacity=0.7,line width=0.48pt] (axis cs:5.0902,0) rectangle (axis cs:5.2544,2);
\draw[draw=black,fill=darkorange,opacity=0.7,line width=0.48pt] (axis cs:5.2544,0) rectangle (axis cs:5.4186,1);
\draw[draw=black,fill=darkorange,opacity=0.7,line width=0.48pt] (axis cs:5.4186,0) rectangle (axis cs:5.5828,2);
\draw[draw=black,fill=darkorange,opacity=0.7,line width=0.48pt] (axis cs:5.5828,0) rectangle (axis cs:5.747,1);
\draw[draw=black,fill=darkorange,opacity=0.7,line width=0.48pt] (axis cs:5.747,0) rectangle (axis cs:5.9112,1);
\draw[draw=black,fill=darkorange,opacity=0.7,line width=0.48pt] (axis cs:5.9112,0) rectangle (axis cs:6.0754,9);
\draw[draw=black,fill=darkorange,opacity=0.7,line width=0.48pt] (axis cs:6.0754,0) rectangle (axis cs:6.2396,46);
\draw[draw=black,fill=darkorange,opacity=0.7,line width=0.48pt] (axis cs:6.2396,0) rectangle (axis cs:6.4038,0);
\draw[draw=black,fill=darkorange,opacity=0.7,line width=0.48pt] (axis cs:6.4038,0) rectangle (axis cs:6.568,2);
\draw[draw=black,fill=darkorange,opacity=0.7,line width=0.48pt] (axis cs:6.568,0) rectangle (axis cs:6.7322,0);
\draw[draw=black,fill=darkorange,opacity=0.7,line width=0.48pt] (axis cs:6.7322,0) rectangle (axis cs:6.8964,1);
\draw[draw=black,fill=darkorange,opacity=0.7,line width=0.48pt] (axis cs:6.8964,0) rectangle (axis cs:7.0606,0);
\draw[draw=black,fill=darkorange,opacity=0.7,line width=0.48pt] (axis cs:7.0606,0) rectangle (axis cs:7.2248,0);
\draw[draw=black,fill=darkorange,opacity=0.7,line width=0.48pt] (axis cs:7.2248,0) rectangle (axis cs:7.389,0);
\draw[draw=black,fill=darkorange,opacity=0.7,line width=0.48pt] (axis cs:7.389,0) rectangle (axis cs:7.5532,0);
\draw[draw=black,fill=darkorange,opacity=0.7,line width=0.48pt] (axis cs:7.5532,0) rectangle (axis cs:7.7174,0);
\draw[draw=black,fill=darkorange,opacity=0.7,line width=0.48pt] (axis cs:7.7174,0) rectangle (axis cs:7.8816,0);
\draw[draw=black,fill=darkorange,opacity=0.7,line width=0.48pt] (axis cs:7.8816,0) rectangle (axis cs:8.0458,0);
\draw[draw=black,fill=darkorange,opacity=0.7,line width=0.48pt] (axis cs:8.0458,0) rectangle (axis cs:8.21,1);
\end{axis}

\end{tikzpicture}
