# Supplementary material for: Integrated Balanced and Staggered Routing in Autonomous Mobility-on-Demand Systems
Source: arXiv:2506.19722 source file (2025-06-24)
Supplement: Supplementary file 2 [file boxplot_total_delays_HC.tex]

% This file was created with tikzplotlib v0.10.1.
\begin{tikzpicture}

\definecolor{darkgray176}{RGB}{176,176,176}

\begin{axis}[
height=\MathAppendixHeight,
tick align=outside,
tick pos=left,
width=\MathAppendixWidth,
x grid style={darkgray176},
xlabel={[hrs]},
xmajorgrids,
xmin=0, xmax=30,
xtick style={color=black},
y dir=reverse,
ymin=-0.5, ymax=0.5,
ytick=\empty,
]
\path [draw=black, fill=white, semithick]
(axis cs:4.47641363888889,-0.4)
--(axis cs:4.47641363888889,0.4)
--(axis cs:14.8342691388889,0.4)
--(axis cs:14.8342691388889,-0.4)
--(axis cs:4.47641363888889,-0.4)
--cycle;
\addplot [semithick, black]
table {%
4.47641363888889 0
1.82075486111111 0
};
\addplot [semithick, black]
table {%
14.8342691388889 0
26.0536160833333 0
};
\addplot [semithick, black]
table {%
1.82075486111111 -0.2
1.82075486111111 0.2
};
\addplot [semithick, black]
table {%
26.0536160833333 -0.2
26.0536160833333 0.2
};
\addplot [black, opacity=0.6, mark=o, mark size=0.5, mark options={solid,fill opacity=0}, only marks]
table {%
45.2951990555556 0
40.9132319722222 0
42.6787258333333 0
};
\addplot [semithick, black]
table {%
6.51872152777778 -0.4
6.51872152777778 0.4
};
\end{axis}

\end{tikzpicture}
