# Supplementary material for: Integrated Balanced and Staggered Routing in Autonomous Mobility-on-Demand Systems
Source: arXiv:2506.19722 source file (2025-06-24)
Supplement: Supplementary file 3 [file boxplot_total_delays_LC.tex]

% This file was created with tikzplotlib v0.10.1.
\begin{tikzpicture}

\definecolor{darkgray153}{RGB}{153,153,153}
\definecolor{darkgray176}{RGB}{176,176,176}

\begin{axis}[
height=\MathAppendixHeight,
tick align=outside,
tick pos=left,
width=\MathAppendixWidth,
x grid style={darkgray176},
xlabel={[hrs]},
xmajorgrids,
xmin=0, xmax=2,
xtick style={color=black},
y dir=reverse,
ymin=-0.5, ymax=0.5,
ytick=\empty,
]
\path [draw=darkgray153, fill=white, thick]
(axis cs:0.920795048611111,-0.4)
--(axis cs:0.920795048611111,0.4)
--(axis cs:1.51656264583333,0.4)
--(axis cs:1.51656264583333,-0.4)
--(axis cs:0.920795048611111,-0.4)
--cycle;
\addplot [thick, darkgray153]
table {%
0.920795048611111 0
0.438657777777778 0
};
\addplot [thick, darkgray153]
table {%
1.51656264583333 0
1.72222983333333 0
};
\addplot [thick, darkgray153]
table {%
0.438657777777778 -0.2
0.438657777777778 0.2
};
\addplot [thick, darkgray153]
table {%
1.72222983333333 -0.2
1.72222983333333 0.2
};
\addplot [black, mark=o, mark size=1, mark options={solid,fill opacity=0,draw=darkgray153}, only marks]
table {%
4.32538769444444 0
23.5366964166667 0
23.5366964166667 0
2.44994880555556 0
};
\addplot [thick, darkgray153]
table {%
1.13507683333333 -0.4
1.13507683333333 0.4
};
\end{axis}

\end{tikzpicture}
